# Supplementary material for: Highly charged Nd$^{9+}$ Ion: A potential candidate of $\upmu$Hz linewidth optical clocks for probing fundamental physics
Source: arXiv:2107.10520 source file (2021-07-22)
Supplement: Supplementary file 1 [file Suppl.pdf]

# I. THE MULTI-REFERENCE CONFIGURATION INTERACTION (MRCI) CALCULATIONS

In the MRCI calculations we consider the $Nd^{9+}$ ion as a many-body system of 59 electrons with the ground state configuration being $[1s^2, ..., 4d^{10}5s^25p^24f]$. Such atomic system can be regarded as the 3-valence (3-val) system with three valence electrons $5p^24f$ above the core $[1s^2, ..., 4d^{10}5s^2]$ or the 5-valence (5-val) system with five valence electrons $5s^25p^24f$ above the core $[1s^2, ..., 4d^{10}]$. We first start with the Dirac-Hartree-Fock (DHF) calculation under the Dirac-Coulomb-Gaunt Hamiltonian, which is given by

$$\hat{H} = \sum_i [c(\vec{\alpha}\cdot\vec{\mathbf{p}})_i + (\beta-1)_i m_0c^2 + V_{iA}] + \sum_{i<j}\left[\frac{1}{r_{ij}} - \frac{1}{2}\frac{\vec{\alpha}_i\cdot\vec{\alpha}_j}{r_{ij}}\right], \quad (1)$$

where $i, j$ denote electrons, $r_{ij}$ is the distance between $i$ and $j$ electrons, $m_0c^2$ is the rest mass energy of an electron with speed of light $c$ and $V_{iA}$ is the nuclear potential with atomic mass number $A$. The last term in Eq.(1) is the Gaunt term that is the leading term of the Breit interaction. Based on the single-electron wavefunctions obtained by the DHF calculation, the MRCI calculation is carried out for both cases (3-val and 5-val systems) by using the KRCI module, a string-based Hamiltonian-direct configuration interaction (CI) program [1–3] in the DIRAC package [4]. The Dyall's uncontracted correlation consistent double-, triple-, and quandruple-$\zeta$ basis sets constructed as linear combinations of Gaussian type orbitals, referred as $X\zeta$ with $X$=2, 3, 4, respectively [5] are adopted, which amounts to {24s;19p;13d;8f;2g}, {30s;24p;16d;11f;3g;2h}, and {35s;30p;19d;13f;5g;3h;2i} functions in the $2\zeta$, $3\zeta$, and $4\zeta$ basis sets, respectively. In the MRCI calculations, the excitation from the active core shells and the valence shells to the virtual orbitals up to $9sp8df6g$ ($s$- and $p$-orbitals with $n\leq9$, $d$- and $f$-orbitals with $n\leq8$, and $g$-orbitals with $n\leq6$) at the $X$=2 basis set, $10sp9df6g7h$ ($s$- and $p$-orbitals with $n\leq10$, $d$- and $f$-orbitals with $n\leq9$, $g$-orbitals with $n\leq6$, and $h$-orbitals with $n\leq7$) at the $X$=3 basis set, and $12sp10df7ghi$ ($s$- and $p$-orbitals with $n\leq12$, $d$- and $f$-orbitals with $n\leq10$, $g$-, $h$-, and $i$-orbitals with $n\leq7$ ) at the $X$=4 basis set, respectively, with higher-lying virtual orbitals being truncated.

The results for the excited energy (EE) are given in Table I and II for the 3-val and 5-val cases, respectively. The influence of the electronic correlation on the computation results is investigated through the hierarchical CI model spaces. First, along with the single and double excitations of the valence electrons, we consider single excitation from the outer core $(4d, 5s)$ ( 12 electrons), referred to as '(core12)', in the 3-val case and $(4d)$ (10 electrons), referred to as '(core10)', in the 5-val case with the remaining inner core electrons frozen. The EE values obtained by the '(core12)' (3-val) and '(core10)' (5-val) MRCI calculations are performed with the $X$=2, 3, 4 basis sets, as given in the 2nd, 3th and 4th columns, respectively. The obtained EE values change with the increasing basis sets, which indicates the possible correction of the results due to a larger basis set, referred as $\Delta_{basis}$. The $\Delta_{basis}$correction is listed in the 7th column, as estimated by the difference in the results for $X = 3$ and $X = 4$ basis sets, i.e., the 3rd and 4th columns.

Next, we consider the single excitation from the outer core $(4s, 4p, 4d, 5s)$ (20 electrons) plus the double excitations from $(4d, 5s)$, referred to '(core20)$_C$' in the 3-val case, and the single excitation from $(4s, 4p, 4d)$ (18 electrons) and additional double excitation from $(4d)$, referred to '(core18)$_C$', in the 5-val case. Along with the single and double excitations from the valence electrons, the '(core18)$_C$' and '(core20)$_C$' model spaces include more core-valence as well as core-core interactions in the MRCI calculation. The results of EE obtained by the '(core18)$_C$' and '(core20)$_C$' calculations with the $X = 2$ basis set are listed in the 5th column. The changes of the results between the '(core12)' and '(core20)$_C$', i.e., the 2nd and 5th columns in Table I, in the 3-val case and those between the '(core10)' and '(core18)$_C$', i.e., the 2nd and 5th columns in Table II, in the 5-val case account for the possible corrections caused by more electronic correlations, referred as $\Delta_C$, which is given in the 8th column.

Further, single, double and triple excitations from the valence electrons are considered along with the single excitation from the small outer core $(4d, 5s)$ in the 3-val case and $(4d)$ in the 5-val case. The EE values obtained by such calculations, referred as '(core12)$_T$' (3-val) and '(core10)$_T$' (5-val), are given in the 6th column. The differential values between '(core12)' and '(core12)$_T$', i.e., the 2nd and 6th columns in Table I, in the 3-val case and those between '(core10)' and '(core10)$_T$', i.e., the 2nd and 6th columns in Table II, in the 5-val case indicate the possible corrections caused by the triple excitation, referred as $\Delta_T$, which is given in the 9th column. The QED interaction is absent in the MRCI method. The QED correction, $\Delta_{QED}$, listed in the 10th column of Table I and II are taken from the AMBiT results.

The final EE value, as listed in the 12th column, is a composite of the EE value obtained by the '(core12)' (3-val) calculation and the '(core10)' (5-val) calculation with the $X = 4$ basis set and the corresponding $\Delta_{basis}$, $\Delta_C$, $\Delta_T$, and $\Delta_{QED}$ corrections. The uncertainties of the final EE values are assigned by rms of $\Delta_{basis}$, $\Delta_C$, $\Delta_T$, and $\Delta_{QED}$, as listed in the 13th column. We find that the 3-val and 5-val calculations give consistent results for the sequence of the energy levels, however, the EE values obtained by the 3-val calculation are smaller 2000-3000cm$^{-1}$ than the results obtained by the 5-val calculation. The 5-val calculation considers more electronic correlations than the 3-val calculation, therefore the results obtained by the 5-val calculation are adopted in this work.

TABLE I: Excited energies (EE) ($cm^{-1}$) of atomic states in $Nd^{9+}$ ion obtained by 3-val MRCI calculation.

| Level | $X$=2 (core12) | $X$=3 (core12) | $X$=4 (core12) | $X$=2 (core20)$_C$ | $X$=2 (core12)$_T$ | $\Delta_{basis}$ | $\Delta_C$ | $\Delta_T$ | $\Delta_{QED}$ | Final | Uncert. |
|---|---|---|---|---|---|---|---|---|---|---|---|
| (1) | (2) | (3) | (4) | (5) | (6) | (7) | (8) | (9) | (10) | (11) | (12) |
| G0: $(5p^2 4f)^o_{5/2}$ | 0 | 0 | 0 | 0 | 0 | 0 | 0 | 0 | 0 | 0 | 0 |
| G1: $(5p^2 4f)^o_{7/2}$ | 6522 | 6545 | 6570 | 6545 | 6516 | 25 | 23 | -6 | 20 | 6632 | 40 |
| E0: $(5p4f^2)^o_{9/2}$ | 18864 | 21432 | 22812 | 19838 | 18986 | 1380 | 974 | 122 | -157 | 25131 | 1701 |
| E1: $(5p4f^2)^o_{7/2}$ | 21473 | 23294 | 24177 | 22832 | 21582 | 883 | 1360 | 109 | -122 | 26408 | 1630 |
| E2: $(5p4f^2)^o_{11/2}$ | 25086 | 27717 | 29107 | 26859 | 25220 | 1390 | 1773 | 133 | -138 | 32265 | 2261 |
| E3: $(5p4f^2)^o_{9/2}$ | 25552 | 28123 | 29436 | 27035 | 25693 | 1312 | 1483 | 141 | -132 | 32240 | 1990 |
| E4: $(5p4f^2)^o_{5/2}$ | 27366 | 29639 | 30713 | 28449 | 27532 | 1075 | 1082 | 165 | -140 | 32896 | 1541 |
| E5: $(5p4f^2)^o_{3/2}$ | 28166 | 30273 | 31184 | 29648 | 28414 | 912 | 1482 | 248 | -115 | 33711 | 1762 |
| E6: $(5p4f^2)^o_{7/2}$ | 29348 | 31583 | 32748 | 30357 | 29517 | 1165 | 1009 | 169 | -125 | 34967 | 1556 |
| E7: $(5p4f^2)^o_{11/2}$ | 29702 | 32364 | 33715 | 31250 | 29841 | 1351 | 1548 | 139 | -119 | 36633 | 2063 |
| E8: $(5p4f^2)^o_{5/2}$ | 31029 | 33076 | 34066 | 31923 | 31188 | 990 | 894 | 159 | -120 | 35989 | 1349 |
| E9: $(5p4f^2)^o_{13/2}$ | 31076 | 33727 | 35113 | 33572 | 31227 | 1386 | 2496 | 151 | -119 | 39027 | 2861 |

TABLE II: Excited energies (EE) ($cm^{-1}$) of atomic states in $Nd^{9+}$ ion obtained by 5-val MRCI calculation.

| Level | $X$=2 (core10) | $X = 3$ (core10) | $X$=4 (core10) | $X$=2 (core18)$_C$ | $X$=2 (core10)$_T$ | $\Delta_{basis}$ | $\Delta_C$ | $\Delta_T$ | $\Delta_{QED}$ | Final | Uncert. |
|---|---|---|---|---|---|---|---|---|---|---|---|
| (1) | (2) | (3) | (4) | (5) | (6) | (7) | (8) | (9) | (10) | (11) | (12) |
| G0: $(5p^2 4f)^o_{5/2}$ | 0 | 0 | 0 | 0 | 0 | 0 | 0 | 0 | 0 | 0 | 0 |
| G1: $(5p^2 4f)^o_{7/2}$ | 6514 | 6537 | 6554 | 6605 | 6513 | 17 | 91 | -1 | 20 | 6681 | 95 |
| E0: $(5p4f^2)^o_{9/2}$ | 16462 | 18932 | 20076 | 18395 | 16649 | 1144 | 1932 | 187 | -140 | 23199 | 2258 |
| E1: $(5p4f^2)^o_{7/2}$ | 19583 | 21585 | 22443 | 21146 | 19780 | 858 | 1563 | 198 | -81 | 24982 | 1796 |
| E2: $(5p4f^2)^o_{11/2}$ | 22631 | 25172 | 26310 | 24761 | 22903 | 1138 | 2131 | 272 | -112 | 29738 | 2433 |
| E3: $(5p4f^2)^o_{9/2}$ | 22875 | 25422 | 26504 | 24733 | 23206 | 1082 | 1858 | 332 | -95 | 29680 | 2177 |
| E4: $(5p4f^2)^o_{5/2}$ | 25150 | 27497 | 28488 | 26009 | 25463 | 991 | 859 | 313 | -59 | 30592 | 1350 |
| E5: $(5p4f^2)^o_{3/2}$ | 26931 | 28189 | 29043 | 27940 | 26361 | 854 | 1009 | -569 | -52 | 30284 | 1440 |
| E6: $(5p4f^2)^o_{7/2}$ | 27116 | 29324 | 30321 | 28116 | 27243 | 997 | 1000 | 126 | -44 | 32400 | 1418 |
| E7: $(5p4f^2)^o_{11/2}$ | 28734 | 29520 | 30623 | 30717 | 27403 | 1103 | 1983 | -1331 | -69 | 32309 | 2632 |
| E8: $(5p4f^2)^o_{5/2}$ | 29321 | 30920 | 31842 | 30095 | 28964 | 922 | 774 | -357 | -90 | 33091 | 1259 |
| E9: $(5p4f^2)^o_{13/2}$ | 29942 | 31166 | 32279 | 32215 | 29015 | 1113 | 2273 | -927 | -101 | 34637 | 2697 |

## II. THE CONFIGURATION INTERACTION WITH MANY-BODY PERTURBATION THEORY (CI+MBPT) CALCULATIONS

The CI+MBPT method is a hybrid approach combining CI that takes into account an interaction between valence electrons and a method accounting for core-valence correlations using an MBPT operator [6, 7]. In this work, the CI+MBPT calculation is implemented by using the AMBiT code [8]. The first step is to solve the Dirac-Hartree-Fock (DHF) solution for core and valence electrons in the $V^N$, $V^{N-1}$, or $V^{N-M}$ approximations, where $N$ is the number of electrons and $M$ is the number of valence electrons. In either choice of potential, the resulting one-electron Dirac-Fock operator is

$$h_{DF} = c\vec{\alpha}\cdot\mathbf{\vec{p}} + (\beta+1)c^2 - \frac{Z}{r} + V^{DF}, \qquad (2)$$

where $\vec{\alpha}$ and $\beta$ are Dirac matrices, and $V^{DF}$ is either of $V^N$, $V^{N-1}$, or $V^{N-M}$. The Breit and QED interactions are written into the Dirac-Fock operator. The Breit includes both Gaunt and retardation terms in the frequency-independent limit by

$$B_{ij} = -\frac{1}{r_{ij}}(\vec{\alpha}_i\cdot\vec{\alpha}_j + (\vec{\alpha}_i\cdot\mathbf{\vec{r}}_{ij})(\vec{\alpha}_j\cdot\mathbf{\vec{r}}_{ij})/r_{ij}^2), \qquad (3)$$

and the QED interaction adopts the radiative potential method originally developed by Flambaum and Ginges [9]. The remaining valence and virtual orbitals are con-

TABLE III: Excited energies (EE) ($cm^{-1}$) of atomic states in $Nd^{9+}$ ion obtained by 3-val and 5-val AMBiT calculations under $V^{N-M}$ and $V^{N}$ potentials, where $M$=3 and 5 for 3-val and 5-val cases, respectively .

| Level | 3-val VN-3 | | 3-val VN | | 5-val VN-5 | | 5-val VN | |
|---|---|---|---|---|---|---|---|---|
| | EE($cm^{-1}$) | $g_j$ factor | EE($cm^{-1}$) | $g_j$ factor | EE($cm^{-1}$) | $g_j$ factor | EE($cm^{-1}$) | $g_j$ factor |
| G0: $(5p^2 4f)^o_{5/2}$ | 0 | 0.838 | 0 | 0.840 | 0 | 0.836 | 0 | 0.838 |
| G1: $(5p^2 4f)^o_{7/2}$ | 6465 | 1.155 | 6473 | 1.156 | 6648 | 1.155 | 6392 | 1.157 |
| E0: $(5p4f^2)^o_{9/2}$ | 13606 | 0.813 | 17478 | 0.814 | 17229 | 0.811 | 18994 | 0.813 |
| E1: $(5p4f^2)^o_{7/2}$ | 16903 | 0.812 | 20040 | 0.827 | 20523 | 0.817 | 21640 | 0.828 |
| E2: $(5p4f^2)^o_{11/2}$ | 19803 | 1.015 | 23691 | 1.015 | 23582 | 1.014 | 25154 | 1.015 |
| E3: $(5p4f^2)^o_{9/2}$ | 19908 | 1.038 | 23632 | 1.040 | 23855 | 1.039 | 25135 | 1.041 |
| E4: $(5p4f^2)^o_{5/2}$ | 21256 | 0.663 | 24675 | 0.698 | 24796 | 0.681 | 26001 | 0.739 |
| E5: $(5p4f^2)^o_{3/2}$ | 21979 | 0.747 | 24671 | 0.805 | 25584 | 0.765 | 26386 | 0.793 |
| E6: $(5p4f^2)^o_{7/2}$ | 23620 | 1.021 | 27002 | 1.005 | 27195 | 1.010 | 28253 | 1.002 |
| E7: $(5p4f^2)^o_{11/2}$ | 23970 | 1.184 | 27752 | 1.183 | 28121 | 1.185 | 29200 | 1.185 |
| G2: $(5p^2 4f)^o_{5/2}$ | 27271 | 1.169 | 27627 | 0.952 | 28244 | 1.002 | 28158 | 0.877 |
| E8: $(5p4f^2)^o_{5/2}$ | 24839 | 0.942 | 28325 | 1.131 | 28911 | 1.096 | 29699 | 1.167 |
| E9: $(5p4f^2)^o_{13/2}$ | 25688 | 1.150 | 29577 | 1.150 | 29688 | 1.150 | 31042 | 1.149 |

TABLE IV: Energies (EE) ($cm^{-1}$), lifetime $\tau$ (s), Landé $g_j$ factor, hyperfine structure constant $A$ (MHz), electric quadrupole moment $\Theta$ (a.u.), and relativistic coefficient $q$ ($cm^{-1}$) for variation of fine structure constant in $Nd^{9+}$ ion obtained by MRCI and AMBiT calculations.

| Level | EE | | $\tau$ | | $g_j$ | | A | | $\Theta$ | | $q$ | |
|---|---|---|---|---|---|---|---|---|---|---|---|---|
| | MRCI | AMBiT | MRCI | AMBiT | MRCI | AMBiT | MRCI | AMBiT | MRCI | AMBiT | MRCI | AMBiT |
| G0: $(5p^2 4f)^o_{5/2}$ | 0 | 0 | | | 0.830 | 0.838 | -376 | -352 | 0.019 | 0.006 | | |
| G1: $(5p^2 4f)^o_{7/2}$ | 6681 | 6392 | 0.23 | 0.47 | 1.156 | 1.157 | -175 | -169 | -0.044 | 0.009 | 28462 | 30447 |
| E0: $(5p4f^2)^o_{9/2}$ | 23199 | 18994 | 154 | 392 | 0.808 | 0.813 | -1086 | -1042 | -0.103 | 0.101 | 441457 | 473472 |
| E1: $(5p4f^2)^o_{7/2}$ | 24982 | 21640 | 0.08 | 0.13 | 0.829 | 0.828 | 2 | 86 | 0.082 | 0.082 | 402549 | 434439 |
| E2: $(5p4f^2)^o_{11/2}$ | 29738 | 25154 | 0.16 | 0.32 | 1.011 | 1.015 | -854 | -814 | 0.076 | 0.064 | 473150 | 506634 |
| E3: $(5p4f^2)^o_{9/2}$ | 29680 | 25135 | 0.65 | 1.91 | 1.040 | 1.041 | 192 | 228 | -0.098 | 0.091 | 470982 | 500115 |
| E4: $(5p4f^2)^o_{5/2}$ | 30592 | 26001 | 0.05 | 0.01 | 0.676 | 0.739 | -1352 | -1326 | 0.032 | 0.023 | 433796 | 458656 |
| E5: $(5p4f^2)^o_{3/2}$ | 30284 | 26386 | 0.12 | 0.07 | 0.726 | 0.793 | 1215 | 1051 | -0.034 | 0.032 | 411632 | 380313 |
| G2: $(5p4f^2)^o_{7/2}$ | | 28158 | | 0.01 | | 0.877 | | -152 | | 0.175 | | |
| E6: $(5p4f^2)^o_{11/2}$ | 32400 | 28253 | 0.03 | 0.02 | 1.018 | 1.002 | -437 | -579 | -0.101 | 0.118 | 468998 | 474051 |
| E7: $(5p^2 4f)^o_{5/2}$ | 32309 | 29200 | 0.66 | 1.31 | 1.187 | 1.185 | 307 | 274 | 0.091 | 0.079 | 464518 | 525655 |
| E8: $(5p4f^2)^o_{5/2}$ | 33091 | 29699 | 0.03 | 0.15 | 1.152 | 1.167 | 502 | 581 | 0.079 | 0.085 | 497006 | |
| E9: $(5p4f^2)^o_{13/2}$ | 34637 | 31042 | 0.18 | 0.36 | 1.144 | 1.1494 | -748 | -703 | -0.040 | 0.009 | 418591 | |

structed as a linear combination of B-spline basis functions. In the next version of the AMBiT code, the CI-space of CSFs are formed by allowing an arbitrary number of electron and/or hole excitations from a set of 'leading configuration' up to some maximum principal quantum number, $n$, and orbital angular momentum, $l$. The AMBiT code implements a new approach, referred as 'emu CI', that can reduce the computational cost associated with CI further. In the emu CI approach, in addition to the 'large-side' CSFs, there are 'small-side' CSFs, formed by allowing electron and/or hole-excitations from a set of leading configurations up to some $n$ and $l$ that can be less that those for large-side CSFs. Finally, the MBPT operator and corrections to energies are implemented in the AMBiT code that can include the core-valence interaction perturbatively.

In the 3-val AMBiT calculation, the DHF calculation is carried out with both $V^N$ and $V^{N-3}$ potentials. The valence basis set is chosen to be 20*spdf* that includes *s*-, *p*-, *d*-, and *f*-orbitals with $n < 20$. The $5p^2 4f$ and $5p4f^2$ configurations consists of the set of leading configuration. The single and double excitations from the leading configurations up to 10*spdf* and additional single excitations up to 20*spdf* comprise the large-side CSFs of the CI space. The small-side CSFs are constructed by allowing the single and double excitations from the leading con-

figurations up to 6*spdf* and additional single excitation up to 20*spdf*. In the 5-val AMBiT calculations, we adopt a smaller valence basis set 15*spdf*. The DHF calculation is conducted with both $V^N$ and $V^{N-5}$ potentials. The leading configurations are $5s^25p^24f$ and $5s^25p4f^2$. The single and double excitation from the leading configurations up to 10*spdf* and additional single excitation to 15*spdf* consist of the large-side CSFs, while the small-side CSFs include the single and double excitation from the leading configurations up to 6*spdf* and additional single excitation to 8*spdf* in order to control the size of the CI space for the 5-val system for a reasonable scale. In all AMBiT calculations, hole excitations are neglected and the MBPT calculations are performed with all one-, two-, and three-body MBPT diagrams included based on the 30*spdfg* basis.

In Table III we summarize the results of EE obtained by the AMBiT calculations. While the 3-val and 5-val calculations give the consistent prediction to the energy levels of the atomic states in the $Nd^{9+}$ ion, the 3-val calculation sees an obvious underestimation of EE as compared with the 5-val calculation, and such tendency is dependent on the choice of the $V^{N-M}$ and $V^N$ potentials. The underestimation of EE is more sophisticate in the case of the $V^{N-M}$ potential than of the $V^N$ potential. The results of the 5-val AMBiT calculation with the $V^N$ potential are more close to the MRCI results. However, because of the finite size of the CI space and the absence of hole excitations, it is difficult for us to estimate the uncertainty of the energy values within the AMBiT calculations. In Table IV we compared the MRCI and AMBiT results for the EE, lifetime $\tau$, Landé $g_j$ factor, hyperfine structure constant $A$, electric quadrupole moment $\Theta$, and relativistic coefficient $q$ for variation of the fine-structure constant for our interested atomic states in the $Nd^{9+}$ ion. Such comparison shows the globally excellent agreement. Quantitative agreement between the MRCI and AMBiT calculations needs more sufficient electronic correlation to be implemented within such two methods, which will be pursued in the future.

## III. THE M1, E2 TRANSITION RATES AND LIFETIME

To ascertain the feasibility of considering the ions of our interest for atomic clocks, we calculate the lifetimes ($\tau_f$) of the excited states. For this purpose, we determine the transition wavelength and transition probabilities for the considered state. The transition probabilities of the $f \to i$ transition due to the first three lower-order channels are evaluated using the expressions

$$A_{fi}^{E1} = \frac{2.02613 \times 10^{18}}{(2J_f+1)\lambda_{fi}^3} S_{fi}^{E1}, \quad (4)$$

$$A_{fi}^{M1} = \frac{2.69735 \times 10^{13}}{(2J_f+1)\lambda_{fi}^3} S_{fi}^{M1} \quad (5)$$

and

$$A_{fi}^{E2} = \frac{1.11995 \times 10^{18}}{(2J_f+1)\lambda_{fi}^5} S_{fi}^{E2}, \quad (6)$$

where $\lambda_{fi}$ (in $\mathring{A}$) is the transition wavelength between the upper state $f$ and the down state $i$, and $J$ represents angular momentum of the state, $S_{fi}^{O} = |\langle J_f||\mathbf{O}||J_i\rangle|^2$ known as the line strength due to the transition operator $O$ of the corresponding channel that are used in atomic units (a.u.). Accumulating all possible transition probabilities from the $f$ state, the lifetime ($\tau_f$) of this state is determined by

$$\tau_f = \frac{1}{\sum_{i,O} A_{fi}^{O}}. \quad (7)$$

These values are obtained in second ($s$). Since the $5p^24f$ and $5p4f^2$ configurations have the same odd parity, the E1 transition between them is forbidden, and therefore only the M1 and E2 transitions need to be considered. We present the values of $\lambda$, $S^{M1}$, $S^{E2}$, $A^{M1}$, and $A^{E2}$ values for different transition channels from our interested excited states obtained by the MRCI calculation in Table V and the AMBiT calculation in Table VI. The excellent agreement between the MRCI and AMBiT results proves our prediction for the lifetime of the excited states in the $Nd^{9+}$ ion.

TABLE V: Lifetime $\tau_f$ of low lying states, transition wavelength $\lambda$, M1 and E2 line strengths $S_{fi}^{M1}$ and $S_{fi}^{E2}$, M1 and E2 transition rates $A_{fi}^{M1}$ and $A_{fi}^{E2}$, total transition rate $A_{fi}^{T} = A_{fi}^{M1} + A_{fi}^{E2}$, and branch ratio (BR), obtained by 5-val '(core10)' MRCI calculation with $X = 4$ basis set corresponding to 4-th column in Table II.

| up state ($f$) | $\tau_f$ (s) | down state ($i$) | $\lambda$ ($\mathring{A}$) | $S_{fi}^{M1}$ (a.u.) | $S_{fi}^{E2}$ (a.u.) | $A_{fi}^{M1}$ (/s) | $A_{fi}^{E2}$ (/s) | $A_{fi}^{T}$ (/s) | BR |
|---|---|---|---|---|---|---|---|---|---|
| G1: $(5p^24f)^o_{7/2}$ | 0.23 | G0: $(5p^24f)^o_{5/2}$ | 15257 | 4.59E+00 | 2.97E-05 | 4.30E+00 | 5.03E-09 | 4.32E+00 | 1.00 |
| E0: $(5p4f^2)^o_{9/2}$ | 154.00 | G0: $(5p^24f)^o_{5/2}$ | 4981 | 0.00E+00 | 1.76E-01 | 0.00E+00 | 6.45E-03 | 6.45E-03 | 0.99 |
| | | G1: $(5p^24f)^o_{7/2}$ | 7395 | 3.37E-06 | 3.71E-03 | 2.20E-05 | 1.88E-05 | 4.10E-05 | 0.01 |

| | | | | | | | | | |
|---|---|---|---|---|---|---|---|---|---|
| E1: $(5p4f^2)^o_{7/2}$ | 0.08 | G0: $(5p^24f)^o_{5/2}$ | 4456 | 3.24E-01 | 7.86E-02 | 1.20E+01 | 6.27E-03 | 1.22E+01 | 0.95 |
| | | G1: $(5p^24f)^o_{7/2}$ | 6294 | 4.71E-02 | 4.45E-02 | 6.30E-01 | 6.31E-04 | 6.32E-01 | 0.05 |
| | | E0: $(5p4f^2)^o_{9/2}$ | 42253 | 2.79E-01 | 7.08E-03 | 1.20E-02 | 7.36E-09 | 1.23E-02 | 0.00 |
| E2: $(5p4f^2)^o_{11/2}$ | 0.16 | G0: $(5p^24f)^o_{5/2}$ | 3801 | 0.00E+00 | 0.00E+00 | 0.00E+00 | 0.00E+00 | 0.00E+00 | 0.00 |
| | | G1: $(5p^24f)^o_{7/2}$ | 5062 | 0.00E+00 | 7.06E-02 | 0.00E+00 | 1.98E-03 | 1.98E-03 | 0.00 |
| | | E0: $(5p4f^2)^o_{9/2}$ | 16043 | 1.17E+01 | 2.03E-01 | 6.30E+00 | 1.78E-05 | 6.28E+00 | 1.00 |
| | | E1: $(5p4f^2)^o_{7/2}$ | 25863 | 0.00E+00 | 4.44E-01 | 0.00E+00 | 3.58E-06 | 3.58E-06 | 0.00 |
| E3: $(5p4f^2)^o_{9/2}$ | 0.65 | G0: $(5p^24f)^o_{5/2}$ | 3773 | 0.00E+00 | 6.28E-03 | 0.00E+00 | 9.20E-04 | 9.20E-04 | 0.00 |
| | | G1: $(5p^24f)^o_{7/2}$ | 5013 | 6.72E-03 | 2.46E-01 | 1.40E-01 | 8.70E-03 | 1.51E-01 | 0.10 |
| | | E0: $(5p4f^2)^o_{9/2}$ | 15559 | 2.56E-01 | 1.57E-02 | 1.80E-01 | 1.93E-06 | 1.81E-01 | 0.12 |
| | | E1: $(5p4f^2)^o_{7/2}$ | 24627 | 6.75E+00 | 2.39E-01 | 1.20E+00 | 2.96E-06 | 1.21E+00 | 0.78 |
| | | E2: $(5p4f^2)^o_{11/2}$ | 515138 | 2.49E+00 | 1.11E-02 | 4.90E-05 | 3.42E-14 | 4.86E-05 | 0.00 |
| E4: $(5p4f^2)^o_{5/2}$ | 0.05 | G0: $(5p^24f)^o_{5/2}$ | 3510 | 1.92E-01 | 6.34E-02 | 2.00E+01 | 2.22E-02 | 1.98E+01 | 0.99 |
| | | G1: $(5p^24f)^o_{7/2}$ | 4559 | 6.21E-04 | 1.05E-03 | 2.90E-02 | 9.94E-05 | 2.92E-02 | 0.00 |
| | | E0: $(5p4f^2)^o_{9/2}$ | 11888 | 0.00E+00 | 1.81E-01 | 0.00E+00 | 1.42E-04 | 1.42E-04 | 0.00 |
| | | E1: $(5p4f^2)^o_{7/2}$ | 16543 | 1.34E-01 | 1.44E-02 | 1.30E-01 | 2.17E-06 | 1.32E-01 | 0.01 |
| | | E2: $(5p4f^2)^o_{11/2}$ | 45907 | 0.00E+00 | 0.00E+00 | 0.00E+00 | 0.00E+00 | 0.00E+00 | 0.00 |
| | | E3: $(5p4f^2)^o_{9/2}$ | 50398 | 0.00E+00 | 8.63E-03 | 0.00E+00 | 4.95E-09 | 4.95E-09 | 0.00 |
| E5: $(5p4f^2)^o_{3/2}$ | 0.12 | G0: $(5p^24f)^o_{5/2}$ | 3443 | 5.06E-02 | 7.48E-02 | 8.30E+00 | 4.32E-02 | 8.32E+00 | 1.00 |
| | | G1: $(5p^24f)^o_{7/2}$ | 4447 | 0.00E+00 | 1.12E-01 | 0.00E+00 | 1.81E-02 | 1.81E-02 | 0.00 |
| | | E0: $(5p4f^2)^o_{9/2}$ | 11153 | 0.00E+00 | 0.00E+00 | 0.00E+00 | 0.00E+00 | 0.00E+00 | 0.00 |
| | | E1: $(5p4f^2)^o_{7/2}$ | 15153 | 0.00E+00 | 2.69E-02 | 0.00E+00 | 9.42E-06 | 9.42E-06 | 0.00 |
| | | E2: $(5p4f^2)^o_{11/2}$ | 36589 | 0.00E+00 | 0.00E+00 | 0.00E+00 | 0.00E+00 | 0.00E+00 | 0.00 |
| | | E3: $(5p4f^2)^o_{9/2}$ | 39386 | 0.00E+00 | 0.00E+00 | 0.00E+00 | 0.00E+00 | 0.00E+00 | 0.00 |
| | | E4: $(5p4f^2)^o_{5/2}$ | 180264 | 4.03E-01 | 3.81E-04 | 4.60E-04 | 5.60E-13 | 4.59E-04 | 0.00 |
| E6: $(5p4f^2)^o_{7/2}$ | 0.03 | G0: $(5p^24f)^o_{5/2}$ | 3298 | 3.22E-01 | 1.22E-01 | 3.00E+01 | 4.39E-02 | 3.00E+01 | 0.93 |
| | | G1: $(5p^24f)^o_{7/2}$ | 4208 | 2.95E-02 | 1.84E-02 | 1.30E+00 | 1.96E-03 | 1.32E+00 | 0.04 |
| | | E0: $(5p4f^2)^o_{9/2}$ | 9761 | 2.53E-02 | 1.23E-02 | 9.10E-02 | 1.95E-05 | 9.08E-02 | 0.00 |
| | | E1: $(5p4f^2)^o_{7/2}$ | 12693 | 2.98E-01 | 1.75E-01 | 4.90E-01 | 7.44E-05 | 4.87E-01 | 0.02 |
| | | E2: $(5p4f^2)^o_{11/2}$ | 24928 | 0.00E+00 | 2.06E-03 | 0.00E+00 | 3.00E-08 | 3.00E-08 | 0.00 |
| | | E3: $(5p4f^2)^o_{9/2}$ | 26195 | 1.20E+00 | 6.66E-03 | 2.20E-01 | 7.56E-08 | 2.23E-01 | 0.01 |
| | | E4: $(5p4f^2)^o_{5/2}$ | 54547 | 4.88E+00 | 1.48E-02 | 1.00E-01 | 4.30E-09 | 1.00E-01 | 0.00 |
| | | E5: $(5p4f^2)^o_{3/2}$ | 78213 | 0.00E+00 | 1.04E-02 | 0.00E+00 | 4.98E-10 | 4.98E-10 | 0.00 |
| E7: $(5p4f^2)^o_{11/2}$ | 0.66 | G0: $(5p^24f)^o_{5/2}$ | 3266 | 0.00E+00 | 0.00E+00 | 0.00E+00 | 0.00E+00 | 0.00E+00 | 0.00 |
| | | G1: $(5p^24f)^o_{7/2}$ | 4155 | 0.00E+00 | 1.57E-01 | 0.00E+00 | 1.19E-02 | 1.19E-02 | 0.01 |
| | | E0: $(5p4f^2)^o_{9/2}$ | 9482 | 1.29E-01 | 2.37E-03 | 3.40E-01 | 2.89E-06 | 3.37E-01 | 0.22 |
| | | E1: $(5p4f^2)^o_{7/2}$ | 12225 | 0.00E+00 | 4.31E-03 | 0.00E+00 | 1.47E-06 | 1.47E-06 | 0.00 |
| | | E2: $(5p4f^2)^o_{11/2}$ | 23182 | 3.90E-02 | 6.26E-03 | 7.00E-03 | 8.73E-08 | 6.97E-03 | 0.00 |
| | | E3: $(5p4f^2)^o_{9/2}$ | 24275 | 7.41E+00 | 2.03E-02 | 1.20E+00 | 2.24E-07 | 1.15E+00 | 0.76 |
| | | E4: $(5p4f^2)^o_{5/2}$ | 46832 | 0.00E+00 | 0.00E+00 | 0.00E+00 | 0.00E+00 | 0.00E+00 | 0.00 |
| | | E5: $(5p4f^2)^o_{3/2}$ | 63269 | 0.00E+00 | 0.00E+00 | 0.00E+00 | 0.00E+00 | 0.00E+00 | 0.00 |
| | | E6: $(5p4f^2)^o_{7/2}$ | 331128 | 0.00E+00 | 3.28E-02 | 0.00E+00 | 7.69E-13 | 7.69E-13 | 0.00 |
| E8: $(5p4f^2)^o_{5/2}$ | 0.03 | G0: $(5p^24f)^o_{5/2}$ | 3141 | 2.18E-01 | 2.00E-03 | 3.10E+01 | 1.22E-03 | 3.13E+01 | 0.86 |
| | | G1: $(5p^24f)^o_{7/2}$ | 3955 | 6.32E-02 | 6.77E-02 | 4.50E+00 | 1.31E-02 | 4.56E+00 | 0.13 |
| | | E0: $(5p4f^2)^o_{9/2}$ | 8499 | 0.00E+00 | 7.97E-02 | 0.00E+00 | 3.35E-04 | 3.35E-04 | 0.00 |
| | | E1: $(5p4f^2)^o_{7/2}$ | 10640 | 3.26E-02 | 5.11E-02 | 1.20E-01 | 6.99E-05 | 1.21E-01 | 0.00 |
| | | E2: $(5p4f^2)^o_{11/2}$ | 18076 | 0.00E+00 | 0.00E+00 | 0.00E+00 | 0.00E+00 | 0.00E+00 | 0.00 |
| | | E3: $(5p4f^2)^o_{9/2}$ | 18733 | 0.00E+00 | 1.45E-02 | 0.00E+00 | 1.17E-06 | 1.17E-06 | 0.00 |
| | | E4: $(5p4f^2)^o_{5/2}$ | 29815 | 2.36E-01 | 3.53E-02 | 4.00E-02 | 2.80E-07 | 3.96E-02 | 0.00 |
| | | E5: $(5p4f^2)^o_{3/2}$ | 35724 | 4.09E+00 | 7.91E-02 | 4.00E-01 | 2.54E-07 | 3.99E-01 | 0.01 |
| | | E6: $(5p4f^2)^o_{7/2}$ | 65761 | 7.19E-01 | 2.86E-02 | 1.10E-02 | 4.33E-09 | 1.13E-02 | 0.00 |
| | | E7: $(5p4f^2)^o_{11/2}$ | 82057 | 0.00E+00 | 0.00E+00 | 0.00E+00 | 0.00E+00 | 0.00E+00 | 0.00 |
| E9: $(5p4f^2)^o_{13/2}$ | 0.18 | G0: $(5p^24f)^o_{5/2}$ | 3098 | 0.00E+00 | 0.00E+00 | 0.00E+00 | 0.00E+00 | 0.00E+00 | 0.00 |
| | | G1: $(5p^24f)^o_{7/2}$ | 3887 | 0.00E+00 | 0.00E+00 | 0.00E+00 | 0.00E+00 | 0.00E+00 | 0.00 |

| | | | | | | | | | |
|---|---|---|---|---|---|---|---|---|---|
| | | E0: $(5p4f^2)^o_{9/2}$ | 8195 | 0.00E+00 | 5.20E-03 | 0.00E+00 | 1.13E-05 | 1.13E-05 | 0.00 |
| | | E1: $(5p4f^2)^o_{7/2}$ | 10167 | 0.00E+00 | 0.00E+00 | 0.00E+00 | 0.00E+00 | 0.00E+00 | 0.00 |
| | | E2: $(5p4f^2)^o_{11/2}$ | 16752 | 1.38E+01 | 2.02E-01 | 5.60E+00 | 1.22E-05 | 5.60E+00 | 1.00 |
| | | E3: $(5p4f^2)^o_{9/2}$ | 17315 | 0.00E+00 | 3.04E-01 | 0.00E+00 | 1.56E-05 | 1.56E-05 | 0.00 |
| | | E4: $(5p4f^2)^o_{5/2}$ | 26377 | 0.00E+00 | 0.00E+00 | 0.00E+00 | 0.00E+00 | 0.00E+00 | 0.00 |
| | | E5: $(5p4f^2)^o_{3/2}$ | 30899 | 0.00E+00 | 0.00E+00 | 0.00E+00 | 0.00E+00 | 0.00E+00 | 0.00 |
| | | E6: $(5p4f^2)^o_{7/2}$ | 51077 | 0.00E+00 | 0.00E+00 | 0.00E+00 | 0.00E+00 | 0.00E+00 | 0.00 |
| | | E7: $(5p4f^2)^o_{11/2}$ | 60393 | 1.18E+00 | 2.52E-01 | 1.00E-02 | 2.51E-08 | 1.02E-02 | 0.00 |
| | | E8: $(5p4f^2)^o_{5/2}$ | 228753 | 0.00E+00 | 0.00E+00 | 0.00E+00 | 0.00E+00 | 0.00E+00 | 0.00 |

TABLE VI: Lifetime $\tau_f$ of low lying states, transition wavelength $\lambda$, M1 and E2 line strengths $S^{M1}_{fi}$ and $S^{E2}_{fi}$, M1 and E2 transition rates $A^{M1}_{fi}$ and $A^{E2}_{fi}$, total transition rate $A^T_{fi} = A^{M1}_{fi} + A^{E2}_{fi}$, and branch ratio (BR), obtained by 5-val AMBiT calculation with $V^N$ potential, corresponding to 8-th column in Tabel III.

| up state ($f$) | $\tau_f$ (s) | down state ($i$) | $\lambda$ (Å) | $S^{M1}_{fi}$ (a.u.) | $S^{E2}_{fi}$ (a.u.) | $A^{M1}_{fi}$ (/s) | $A^{E2}_{fi}$ (/s) | $A^T_{fi}$ (/s) | BR |
|---|---|---|---|---|---|---|---|---|---|
| G1: $(5p^24f)^o_{7/2}$ | 0.47 | G0: $(5p^24f)^o_{5/2}$ | 15645 | 4.58E+00 | 4.16E-03 | 2.13E+00 | 3.31E-07 | 2.13E+00 | 1.00 |
| E0: $(5p4f^2)^o_{9/2}$ | 392.06 | G0: $(5p^24f)^o_{5/2}$ | 5265 | 0.00E+00 | 1.28E-01 | 0.00E+00 | 1.86E-03 | 1.86E-03 | 0.73 |
| | | G1: $(5p^24f)^o_{7/2}$ | 7935 | 2.43E-04 | 3.54E-03 | 6.83E-04 | 6.64E-06 | 6.89E-04 | 0.27 |
| E1: $(5p4f^2)^o_{7/2}$ | 0.13 | G0: $(5p^24f)^o_{5/2}$ | 4621 | 4.01E-01 | 2.38E-02 | 7.24E+00 | 8.43E-04 | 7.24E+00 | 0.95 |
| | | G1: $(5p^24f)^o_{7/2}$ | 6558 | 5.28E-02 | 3.24E-02 | 3.33E-01 | 1.99E-04 | 3.33E-01 | 0.04 |
| | | E0: $(5p4f^2)^o_{9/2}$ | 37803 | 2.76E-01 | 1.56E-02 | 9.09E-03 | 1.51E-08 | 9.09E-03 | 0.00 |
| E2: $(5p4f^2)^o_{9/2}$ | 1.91 | G0: $(5p^24f)^o_{5/2}$ | 3978 | 0.00E+00 | 3.38E-02 | 0.00E+00 | 2.00E-03 | 2.00E-03 | 0.00 |
| | | G1: $(5p^24f)^o_{7/2}$ | 5335 | 4.37E-03 | 2.16E-01 | 4.05E-02 | 2.95E-03 | 4.34E-02 | 0.08 |
| | | E0: $(5p4f^2)^o_{9/2}$ | 16284 | 1.80E-01 | 7.71E-03 | 5.85E-02 | 3.97E-07 | 5.85E-02 | 0.11 |
| | | E1: $(5p4f^2)^o_{7/2}$ | 28606 | 7.01E+00 | 2.13E-01 | 4.21E-01 | 6.55E-07 | 4.21E-01 | 0.80 |
| E3: $(5p4f^2)^o_{11/2}$ | 0.32 | G0: $(5p^24f)^o_{5/2}$ | 3975 | 0.00E+00 | 0.00E+00 | 0.00E+00 | 0.00E+00 | 0.00E+00 | 0.00 |
| | | G1: $(5p^24f)^o_{7/2}$ | 5330 | 0.00E+00 | 3.76E-02 | 0.00E+00 | 4.26E-04 | 4.26E-04 | 0.00 |
| | | E0: $(5p4f^2)^o_{9/2}$ | 16234 | 1.16E+01 | 2.44E-01 | 3.15E+00 | 1.05E-05 | 3.15E+00 | 1.00 |
| | | E1: $(5p4f^2)^o_{7/2}$ | 28454 | 0.00E+00 | 4.21E-01 | 0.00E+00 | 1.10E-06 | 1.10E-06 | 0.00 |
| | | E2: $(5p4f^2)^o_{9/2}$ | 5360410 | 2.35E+00 | 1.12E-02 | 1.77E-08 | 1.24E-19 | 1.77E-08 | 0.00 |
| E4: $(5p4f^2)^o_{5/2}$ | 0.01 | G0: $(5p^24f)^o_{5/2}$ | 3846 | 1.99E+00 | 2.08E-02 | 8.50E+01 | 2.52E-03 | 8.50E+01 | 0.99 |
| | | G1: $(5p^24f)^o_{7/2}$ | 5100 | 5.61E-02 | 1.16E-03 | 1.03E+00 | 3.42E-05 | 1.03E+00 | 0.01 |
| | | E0: $(5p4f^2)^o_{9/2}$ | 14272 | 0.00E+00 | 2.14E-04 | 0.00E+00 | 3.68E-08 | 3.68E-08 | 0.00 |
| | | E1: $(5p4f^2)^o_{7/2}$ | 22930 | 4.23E-01 | 5.32E-03 | 8.52E-02 | 8.54E-08 | 8.52E-02 | 0.00 |
| | | E2: $(5p4f^2)^o_{9/2}$ | 115555 | 0.00E+00 | 4.03E-01 | 0.00E+00 | 1.99E-09 | 1.99E-09 | 0.00 |
| | | E3: $(5p4f^2)^o_{11/2}$ | 118101 | 0.00E+00 | 0.00E+00 | 0.00E+00 | 0.00E+00 | 0.00E+00 | 0.00 |
| E5: $(5p4f^2)^o_{3/2}$ | 0.07 | G0: $(5p^24f)^o_{5/2}$ | 3790 | 1.97E-01 | 1.67E-04 | 1.38E+01 | 3.42E-05 | 1.38E+01 | 1.00 |
| | | G1: $(5p^24f)^o_{7/2}$ | 5001 | 0.00E+00 | 1.72E-01 | 0.00E+00 | 8.78E-03 | 8.78E-03 | 0.00 |
| | | E0: $(5p4f^2)^o_{9/2}$ | 13528 | 0.00E+00 | 0.00E+00 | 0.00E+00 | 0.00E+00 | 0.00E+00 | 0.00 |
| | | E1: $(5p4f^2)^o_{7/2}$ | 21067 | 0.00E+00 | 8.78E-03 | 0.00E+00 | 3.39E-07 | 3.39E-07 | 0.00 |
| | | E2: $(5p4f^2)^o_{9/2}$ | 79936 | 0.00E+00 | 0.00E+00 | 0.00E+00 | 0.00E+00 | 0.00E+00 | 0.00 |
| | | E3: $(5p4f^2)^o_{11/2}$ | 81146 | 0.00E+00 | 0.00E+00 | 0.00E+00 | 0.00E+00 | 0.00E+00 | 0.00 |
| | | E4: $(5p4f^2)^o_{5/2}$ | 259325 | 5.33E-01 | 2.82E-02 | 1.17E-04 | 3.84E-12 | 1.17E-04 | 0.00 |
| G2: $(5p^24f)^o_{5/2}$ | 0.01 | G0: $(5p^24f)^o_{5/2}$ | 3551 | 1.57E+00 | 3.11E-02 | 8.52E+01 | 5.61E-03 | 8.52E+01 | 0.99 |
| | | G1: $(5p^24f)^o_{7/2}$ | 4594 | 4.11E-02 | 5.41E-03 | 1.03E+00 | 2.69E-04 | 1.03E+00 | 0.01 |
| | | E0: $(5p4f^2)^o_{9/2}$ | 10913 | 0.00E+00 | 6.01E-01 | 0.00E+00 | 3.95E-04 | 3.95E-04 | 0.00 |
| | | E1: $(5p4f^2)^o_{7/2}$ | 15342 | 5.07E-02 | 3.31E-02 | 3.41E-02 | 3.96E-06 | 3.41E-02 | 0.00 |
| | | E2: $(5p4f^2)^o_{9/2}$ | 33087 | 0.00E+00 | 3.54E-01 | 0.00E+00 | 9.08E-07 | 9.08E-07 | 0.00 |
| | | E3: $(5p4f^2)^o_{11/2}$ | 33292 | 0.00E+00 | 0.00E+00 | 0.00E+00 | 0.00E+00 | 0.00E+00 | 0.00 |
| | | E4: $(5p4f^2)^o_{5/2}$ | 46361 | 1.09E+00 | 4.17E-02 | 2.66E-02 | 1.98E-08 | 2.66E-02 | 0.00 |
| | | E5: $(5p4f^2)^o_{3/2}$ | 56453 | 1.16E-01 | 1.20E-02 | 1.56E-03 | 2.14E-09 | 1.56E-03 | 0.00 |

| | | | | | | | | |
|---|---|---|---|---|---|---|---|---|
| E6: $(5p4f^2)^o_{7/2}$ | 0.02 | G0: $(5p^24f)^o_{5/2}$ | 3539 | 9.66E-01 | 4.74E-01 | 3.88E+01 | 6.37E-02 | 3.89E+01 | 0.89 |
| | | G1: $(5p^24f)^o_{7/2}$ | 4574 | 2.39E-01 | 9.73E-02 | 4.44E+00 | 3.63E-03 | 4.45E+00 | 0.10 |
| | | E0: $(5p4f^2)^o_{9/2}$ | 10800 | 1.50E-02 | 8.70E-04 | 2.12E-02 | 4.42E-07 | 2.12E-02 | 0.00 |
| | | E1: $(5p4f^2)^o_{7/2}$ | 15120 | 4.03E-01 | 2.65E-01 | 2.08E-01 | 2.50E-05 | 2.08E-01 | 0.00 |
| | | E2: $(5p4f^2)^o_{9/2}$ | 32073 | 1.21E+00 | 5.87E-02 | 6.53E-02 | 1.29E-07 | 6.53E-02 | 0.00 |
| | | E3: $(5p4f^2)^o_{11/2}$ | 32266 | 0.00E+00 | 1.62E-02 | 0.00E+00 | 3.46E-08 | 3.46E-08 | 0.00 |
| | | E4: $(5p4f^2)^o_{5/2}$ | 44396 | 4.26E+00 | 5.46E-01 | 8.67E-02 | 2.36E-07 | 8.67E-02 | 0.00 |
| | | E5: $(5p4f^2)^o_{3/2}$ | 53566 | 0.00E+00 | 3.25E-02 | 0.00E+00 | 5.50E-09 | 5.50E-09 | 0.00 |
| | | G2: $(5p^24f)^o_{5/2}$ | 1047436 | 1.27E-01 | 5.48E-01 | 1.96E-07 | 3.25E-14 | 1.96E-07 | 0.00 |
| E7: $(5p4f^2)^o_{11/2}$ | 1.31 | G0: $(5p^24f)^o_{5/2}$ | 3425 | 0.00E+00 | 0.00E+00 | 0.00E+00 | 0.00E+00 | 0.00E+00 | 0.00 |
| | | G1: $(5p^24f)^o_{7/2}$ | 4384 | 0.00E+00 | 7.13E-02 | 0.00E+00 | 2.14E-03 | 2.14E-03 | 0.00 |
| | | E0: $(5p4f^2)^o_{9/2}$ | 9799 | 1.21E-01 | 2.92E-03 | 1.49E-01 | 1.57E-06 | 1.49E-01 | 0.20 |
| | | E1: $(5p4f^2)^o_{7/2}$ | 13227 | 0.00E+00 | 1.77E-03 | 0.00E+00 | 2.13E-07 | 2.13E-07 | 0.00 |
| | | E2: $(5p4f^2)^o_{9/2}$ | 24604 | 7.85E+00 | 2.16E-02 | 6.12E-01 | 1.17E-07 | 6.12E-01 | 0.80 |
| | | E3: $(5p4f^2)^o_{11/2}$ | 24717 | 1.92E-02 | 5.94E-03 | 1.48E-03 | 3.14E-08 | 1.48E-03 | 0.00 |
| | | E4: $(5p4f^2)^o_{5/2}$ | 31259 | 0.00E+00 | 0.00E+00 | 0.00E+00 | 0.00E+00 | 0.00E+00 | 0.00 |
| | | E5: $(5p4f^2)^o_{3/2}$ | 35544 | 0.00E+00 | 0.00E+00 | 0.00E+00 | 0.00E+00 | 0.00E+00 | 0.00 |
| | | G2: $(5p^24f)^o_{5/2}$ | 95964 | 0.00E+00 | 0.00E+00 | 0.00E+00 | 0.00E+00 | 0.00E+00 | 0.00 |
| | | E6: $(5p4f^2)^o_{7/2}$ | 105642 | 0.00E+00 | 1.20E-02 | 0.00E+00 | 4.44E-11 | 4.44E-11 | 0.00 |
| E8: $(5p4f^2)^o_{5/2}$ | 0.15 | G0: $(5p^24f)^o_{5/2}$ | 3367 | 4.84E-03 | 3.39E-03 | 3.08E-01 | 7.98E-04 | 3.09E-01 | 0.05 |
| | | G1: $(5p^24f)^o_{7/2}$ | 4290 | 1.99E-01 | 1.04E-02 | 6.12E+00 | 7.29E-04 | 6.12E+00 | 0.91 |
| | | E0: $(5p4f^2)^o_{9/2}$ | 9341 | 0.00E+00 | 4.95E-04 | 0.00E+00 | 7.09E-07 | 7.09E-07 | 0.00 |
| | | E1: $(5p4f^2)^o_{7/2}$ | 12407 | 1.96E-03 | 3.06E-02 | 2.49E-03 | 1.06E-05 | 2.50E-03 | 0.00 |
| | | E2: $(5p4f^2)^o_{9/2}$ | 21911 | 0.00E+00 | 1.25E-01 | 0.00E+00 | 2.53E-06 | 2.53E-06 | 0.00 |
| | | E3: $(5p4f^2)^o_{11/2}$ | 22001 | 0.00E+00 | 0.00E+00 | 0.00E+00 | 0.00E+00 | 0.00E+00 | 0.00 |
| | | E4: $(5p4f^2)^o_{5/2}$ | 27037 | 7.28E-03 | 1.47E-01 | 8.94E-04 | 1.03E-06 | 8.95E-04 | 0.00 |
| | | E5: $(5p4f^2)^o_{3/2}$ | 30184 | 2.95E+00 | 8.66E-02 | 2.61E-01 | 3.52E-07 | 2.61E-01 | 0.04 |
| | | G2: $(5p^24f)^o_{5/2}$ | 64868 | 6.07E-02 | 1.24E-01 | 5.40E-04 | 1.10E-08 | 5.40E-04 | 0.00 |
| | | E6: $(5p4f^2)^o_{7/2}$ | 69151 | 0.00E+00 | 1.08E-02 | 0.00E+00 | 6.94E-10 | 6.94E-10 | 0.00 |
| | | E7: $(5p4f^2)^o_{11/2}$ | 200191 | 0.00E+00 | 0.00E+00 | 0.00E+00 | 0.00E+00 | 0.00E+00 | 0.00 |
| E9: $(5p4f^2)^o_{13/2}$ | 0.36 | G0: $(5p^24f)^o_{5/2}$ | 3221 | 0.00E+00 | 0.00E+00 | 0.00E+00 | 0.00E+00 | 0.00E+00 | 0.00 |
| | | G1: $(5p^24f)^o_{7/2}$ | 4057 | 0.00E+00 | 0.00E+00 | 0.00E+00 | 0.00E+00 | 0.00E+00 | 0.00 |
| | | E0: $(5p4f^2)^o_{9/2}$ | 8301 | 0.00E+00 | 6.90E-03 | 0.00E+00 | 7.26E-06 | 7.26E-06 | 0.00 |
| | | E1: $(5p4f^2)^o_{7/2}$ | 10636 | 0.00E+00 | 0.00E+00 | 0.00E+00 | 0.00E+00 | 0.00E+00 | 0.00 |
| | | E2: $(5p4f^2)^o_{9/2}$ | 16932 | 0.00E+00 | 3.91E-01 | 0.00E+00 | 1.16E-05 | 1.16E-05 | 0.00 |
| | | E3: $(5p4f^2)^o_{11/2}$ | 16985 | 1.39E+01 | 2.69E-01 | 2.80E+00 | 7.90E-06 | 2.80E+00 | 1.00 |
| | | E4: $(5p4f^2)^o_{5/2}$ | 19839 | 0.00E+00 | 0.00E+00 | 0.00E+00 | 0.00E+00 | 0.00E+00 | 0.00 |
| | | E5: $(5p4f^2)^o_{3/2}$ | 21482 | 0.00E+00 | 0.00E+00 | 0.00E+00 | 0.00E+00 | 0.00E+00 | 0.00 |
| | | G2: $(5p^24f)^o_{5/2}$ | 34678 | 0.00E+00 | 0.00E+00 | 0.00E+00 | 0.00E+00 | 0.00E+00 | 0.00 |
| | | E6: $(5p4f^2)^o_{7/2}$ | 35865 | 0.00E+00 | 0.00E+00 | 0.00E+00 | 0.00E+00 | 0.00E+00 | 0.00 |
| | | E7: $(5p4f^2)^o_{11/2}$ | 54300 | 1.46E+00 | 3.46E-01 | 8.99E-03 | 3.04E-08 | 8.99E-03 | 0.00 |
| | | E8: $(5p4f^2)^o_{5/2}$ | 74511 | 0.00E+00 | 0.00E+00 | 0.00E+00 | 0.00E+00 | 0.00E+00 | 0.00 |

## IV. SYSTEMATICAL ENERGY SHIFTS

**Light shift** We calculate the static electric dipole scalar and tensor polarizabilities $\alpha_S^{E1}$ and $\alpha_T^{E1}$ for the three clock-related states in $Nd^{9+}$ by using the finite-field approach implemented in the MRCI calculations. The results are given in Table VII. The stark shift can be estimated in terms of

$$\delta E_{Stark} = -\delta\alpha_S^{E1}\mathcal{E}^2/2, \tag{8}$$

where $\delta\alpha_S^{E1}$ is the differential values of the static electric dipole scalar polarizabilities, and $\mathcal{E}$ is the typical electric field strength in an ion trap. The fractional DC-stark energy shift of the clock transition is estimated to be $\sim 10^{-23}$ for $\mathcal{E}$=10 $V/m$ given, which is negligibly small. Similarly, the contribution due to the tensor polarizability can be also neglected, since the differential value of $\alpha_T^{E1}$ is also very small. Besides, since the ground $5p^24f$ and excited $5p4f^2$ have the same parity and no E1 transition occurs between them in the optical region, therefore the light shifts due to the E1 interaction should be very small.

**Black-body radiation shift** The differential BBR shift at the room temperature, $T$=300K, due to the E1 channel for the clock transition is estimated using the

TABLE VII: Static electric dipole scalar $\alpha_S^{E1}$, static electric dipole tensor $\alpha_T^{E1}$ and static magnetic dipole polarizabilites $\alpha^{M1}$.

| Level | $\alpha_S^{E1}$ | $\alpha_T^{E1}$ | $\alpha^{M1}$ |
|---|---|---|---|
| G0: $(5p^24f)^o_{5/2}$ | 2.218 | -0.044 | -18.09 |
| G1: $(5p^24f)^o_{7/2}$ | 2.220 | -0.060 | -2.90 |
| E0: $(5p4f^2)^o_{9/2}$ | 2.235 | 0.005 | -29.89 |

expression

$$\delta E_{BBR}^{E1} = -\frac{1}{2}(831.9V/m)^2 \left[\frac{T(K)}{300}\right]^4 \delta\alpha_S^{E1}, \quad (9)$$

and found to be much lower than $10^{-19}$ level. Similarly, the BBR shift due to other dominant M1 channel of the $|\eta\rangle$ state can be estimated using the formula

$$\Delta E_{BBR}^{M1} = -\frac{\mu_0(K_BT)^2}{\pi^2(c\hbar)^3}\sum_\beta \left[|\langle\eta||O^{M1}||\beta\rangle|^2\omega_{\eta\beta} \times \int_0^\infty d\omega \frac{\omega^3}{(\omega_{\eta\beta}^2-\omega^2)(\exp^{\hbar\omega/K_BT}-1)}\right], (10)$$

where $\mu_0$, $K_B$, $\hbar$, and $c$ are the magnetic permeability, Boltzmann's constant, Plank's constant, and speed of light, respectively. The $\langle\eta||O^{M1}||\beta\rangle$ value is calculated for the related fine structure levels. Then, the BBR shift due to the M1 channel is determined as differential values of $\Delta E_{BBR}^{M1}$ between two clock states. We find the the BBR shifts due to E1 and M1 interaction are both around $10^{-19}$ level at room temperature, but the real value should be much lower by least 3-4 orders since the actual temperature of HCIs is usually only a few tens of Kelvin.

**Second-order Zeeman shift** While the first-order Zeeman shift can be eliminated, the second-order Zeeman shift, $\delta E_{Zeem}^{(2)} = -\frac{1}{2}\delta\alpha^{M1}B^2$, in the ion clock needs to be considered, wherein $\delta\alpha^{M1}$ is the differential value of $\alpha^{M1}$ between the clock states, $B$ is the external magnetic field and $\mu_B$ is Bohr magneton. We evaluate $\alpha^{M1}$ for the fine-structure level $|\gamma JM_J\rangle$ as

$$\alpha^{M1}(J) = -\frac{2}{3(2J+1)}\sum_{J'}\frac{|\langle J||O^{M1}||J'\rangle|^2}{E_J - E_{J'}}, \quad (11)$$

wherein $E_{J,J'}$ is the energy. Assuming a typical value of $B$=5 × $10^{-8}$T, $\delta E_{Zeem}^{(2)}/\nu$ is found to be $10^{-24}$ .

**Electric quadrupole shift** The electric quadrupole shift is caused due to the gradient of electric field ($\nabla\mathcal{E}$) experienced by the atomic system during the measurement. This can be estimated by calculating the expectation value of the corresponding interaction Hamiltonian $H_Q = -\nabla\mathcal{E}\cdot\Theta(\gamma, K)$ as

$$\Delta E_{Quad} = \langle\gamma K, M_K = K|H_Q|\gamma K, M_K = K\rangle, (12)$$

TABLE VIII: Wavelength $\lambda$, supperradiant lasing linewidth $\Delta\nu$, differential static electric-dipole and magnetic dipole polarizabilities $\delta\alpha_S^{E1}$ and $\delta\alpha^{M1}$, and prevailing energy shifts including second-order zeeman shift $\delta E_{Zeem}^{(2)}/\nu_0$, DC stark shift $\delta E_{Stark}/\nu_0$, and black-body radiation shifts $\delta E_{BBR}^{E1}/\nu_0$ and $\delta E_{BBR}^{M1}/\nu_0$ through the E1 and M1 channels, where $\nu_0$ is active clock frequency. Number in parenthesis is error in $\lambda$ estimated in term of the MRCI calculations given in Table II.

| Items | $(5p4f^2)^o_{9/2} - (5p^24f)^o_{7/2}$ |
|---|---|
| $\lambda$ (nm) | 605(90) |
| $\Delta\nu$ (μHz) | 2-800 |
| $\delta\alpha_S^{E1}$ (a.u.) | 0.015 |
| $\delta\alpha^{M1}$ (a.u.) | -29.76 |
| $\delta E_{Zeem}^{(2)}/\nu_0$ | 9.89×$10^{-24}$ |
| $\delta E_{Stark}/\nu_0$ | -2.87×$10^{-23}$ |
| $\delta E_{BBR}^{E1}/\nu_0$ | -3.98×$10^{-19}$ |
| $\delta E_{BBR}^{M1}/\nu_0$ | -4.91×$10^{-19}$ |

where $K$ is the angular momentum of the state with its component $M_K$, $\gamma$ represents for other quantum numbers such as parity and $\Theta(\gamma, K)$ is known as quadrupole moment, which is the expectation value of the electric quadrupole operator $\Theta = \frac{e}{2}(3z^2 - r^2)$, of the state. The electric quadrupole shift is a typical systematic effect in the HCI clock since clock states in most HCI candidates possess non-zero $\Theta$. In the case of the $Nd^{9+}$ ion, for a given static electric field for instance being $10^8$V/m$^2$, the electric quadrupole shift could be around $10^{-15}$ level. However, the electric quadrupole shift can be reduced by using experimental techniques, for example, measuring and averaging out the transitions in all the $M$-component directions is capable of suppressing the fractional energy shift due to $\mathcal{E}_{zz}$ down to $10^{-19}$ [10].

## V. REDUCTION OF THE CAVITY PULLING

Frequency pulling of the cavity is suppressed in our bad cavity regime by a factor of $a = \kappa/\Delta\omega_b$, where the cavity dissipation rate $\kappa = 2\pi \times 10$ kHz, and $\Delta\omega_b$ is the inhomogeneous broadening. For a typical experimental condition, we can expect minimum value of $a = 10^3$. In Fig. 1 we illustrate the trajectory of the instability of the clock frequency decreasing with the averaging time for various cases. The blue circle corresponds to the state-of-art single $Al^+$ ion optical clock [11, 12], which shows asymptotical instability $\sigma(t) = 1.2 \times 10^{-15}/\sqrt{\tau}$. A cavity mode of the active clock if operated in a high-finess FP optical cavity as reported the best so far [13] starts from an improved instability like $10^{-14}$, which indicates an excellent short-term instability of $10^{-18}$ for averaging time between 1s-100s, however, turn to continually rise after 100 seconds due to the cavity drift. The trends

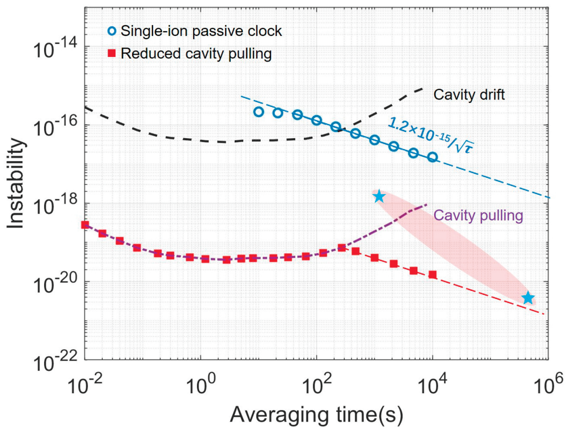


FIG. 1: Drift of the free-running cavity (black dashed line), drift-induced cavity pulling in the bad-cavity regime (purple dash-dot line), instability of the $Al^{+}$ passive optical clock (blue circles), reduced cavity pulling (red squares), and the estimated stability range of the active optical clock (elliptical region) with blue stars represent linewidth of 2 μHz and 800 μHz, respectively.

of the instability of the clock frequency versus the averaging time for the cases of the cavity drift [13] and the cavity pulling (here we assume that the free-running cavity can cause the drift of the clock frequency to decrease three orders of magnitudes, corresponds to the condition of $a = 10^3$) are illustrated by the dashed line and the dash-dot line. We consider that the cavity drift can be reduced technically, for example, by synchronizing to another atomic frequency standard, the drift-induced cavity pulling will maintain the decrease with averaging time going on, and it represents $10^{-20}$-$10^{-21}$ instability for a period of $10^2 - 10^6$ averaging time, as denoted by the red line. For our estimated 2-800 μHz linewidth of the $Nd^{9+}$ active clock, the instability regime is highlighted by the pink shallowed region with two blue stars, corresponding to 2 and 800μHz linewidth, respectively, which is safely located above the red line. This indicates that, when the cavity drift is solved with pulling suppressed, the regained averaging time can ensure that the 2 and 800μHz super-narrow linewidth is reached.


[1] J. Olsen, P. Jørgensen, and J. Simons, Chem. Phys. Lett., **169**, 463 (1990).

[2] T. Fleig, J. Olsen, and L. Visscher, J. Chem. Phys. **119**, 2963 (2003).

[3] T. Fleig, H. J. A. Jensen, J. Olsen, and L. Visscher, J. Chem. Phys. **124** 104106 (2006).

[4] DIRAC, a relativistic ab initio electronic structure program, Release DIRAC13 (2013), written by L. Visscher, H. J. Aa. Jensen, R. Bast, T. Saue, with contributions from V. Bakken, K. G. Dyall, S. Dubillard, U. Ekström, E. Eliav, T. Enevoldsen, E. Faßhauer, T. Fleig, O. Fossgaard, A. S. P. Gomes, T. Helgaker, J. K. Lærdahl, Y. S. Lee, J. Henriksson, M. Iliaš, Ch. R. Jacob, S. Knecht, S. Komorovský, O. Kullie, C. V. Larsen, H. S. Nataraj, P. Norman, G. Olejniczak, J. Olsen, Y. C. Park, J. K. Pedersen, M. Pernpointner, K. Ruud, P. Sałek, B. Schimmelpfennig, J. Sikkema, A. J. Thorvaldsen, J. Thyssen, J. van Stralen, S. Villaume, O. Visser, T. Winther, and S. Yamamoto (see http://www.diracprogram.org).

[5] A.S.P. Gomes, K.G. Dyall and L. Visscher, Theor. Chem. Acc. **127**, 369 (2010).

[6] V.A. Dzuba, V.V. Flambaum, M.G. Kozlov, Phys. Rev. A 54 (1996) 3948.

[7] J.C. Berengut, V.V. Flambaum, M.G. Kozlov, Phys. Rev. A 73 (2006) 012504.

[8] E.V. Kahl and J.C. Berengut, Computer Phys. Comm. **238** 232 (2019).

[9] V.V. Flambaum and J.S.M. Ginges, Phys. Rev. A **72** 052115 (2005).

[10] P. Dubé, A. A. Madej, Z. Zhou, and J. E. Bernard, Phys. Rev. A **87**, 023806 (2013).

[11] K. Beloy, M. I. Bodine, T. Bothwell et al., Nature **591**, 564 (2021).

[12] S. M. Brewer, J.-S. Chen, A. M. Hankin, E. R. Clements, C. W. Chou, D. J. Wineland, D. B. Hume, and D. R. Leibrandt, Phys. Rev. Lett. **123**, 033201 (2019).

[13] D. G. Matei, T. Legero, S. Häfner, C. Grebing, R. Weyrich, W. Zhang, L. Sonderhouse, J. M. Robinson, J. Ye, F. Riehle., and U. Sterr, Phys. Rev. Lett. **118** , 263202 (2017).
